# Supplementary material for: ReFine: Re-randomization before Fine-tuning for Cross-domain Few-shot Learning
Source: arXiv:2205.05282 source file (2022-09-17)
Supplement: Supplementary file 1 [file 08_supplement.tex]

\appendix
\onecolumn
% \section*{Supplement}
% \subsection*{Stability during fine-tuning}
% Prior works have provided the results when fine-tuning is finished. We investigate the fluctuations during fine-tuning and observe that fine-tuning is significantly unstable when few samples are available. Figure XXX describes XXX.

% Furthermore, batch size during fine-tuning is one of the important factors. Figure XXX describes XXX. In the Baseline case, XX, whereas in the Baseline (Body) case, XX.

% Stochastic weight average (SWA) technique

% \subsection*{Fine-tuning parts depending on shot(s)}
% In the case of 1-shot, freezing the pre-trained backbone during fine-tuning is better than updating the entire network. In \cite{bscd_fsl} and \cite{nakamura2019revisiting}, they showed that fine-tuning the entire network is better than fine-tuning only a classifier. However, they did not address 1-shot cases. Figure XXX and XXX describe 1-shot cases and 5-shot cases, respectively. It is believed that XXX.

\section*{Appendix}
\bigskip

\section{Detailed Numbers of Figure 1}\label{appx:detail_of_figure1}

\begin{table}[h]
\caption{Stage-wise 5-way $k$-shot accuracy (\%) of the features from a miniImageNet pre-trained model. An average pooling layer and an auxiliary classifier are attached at the end of each stage of ResNet10.}\label{tab:subnetworks}
\vspace{0.3cm}
\centering{%
\begin{tabular}{c|c|c|cccc|c}
    \toprule
    \multirow{2}{*}{Shot} & \multirow{2}{*}{Aux.} & Same-domain & \multicolumn{5}{c}{Cross-domain (BSCD-FSL)} \\
    \cmidrule{3-8}
     & & miniImageNet & CropDisease & EuroSAT & ISIC & ChestX & Mean \\
    \midrule
    \multirow{4}{*}{1} & Stage1 & 33.79{\stdfont $\pm$.68} & 46.66{\stdfont $\pm$.98} & 46.42{\stdfont $\pm$.82} & 26.77{\stdfont $\pm$.51} & 20.59{\stdfont $\pm$.28} & 35.11 \\
    & Stage2 & 39.31{\stdfont $\pm$.72} & 57.82{\stdfont $\pm$.94} & 54.05{\stdfont $\pm$.86} & 28.01{\stdfont $\pm$.52} & 20.84{\stdfont $\pm$.32} & 40.18 \\
    & Stage3 & 47.28{\stdfont $\pm$.80} & 65.69{\stdfont $\pm$.85} & 61.56{\stdfont $\pm$.90} & 30.07{\stdfont $\pm$.56} & 22.00{\stdfont $\pm$.38} & \textbf{44.83} \\
    & Stage4 & \textbf{51.88{\stdfont $\pm$.80}} & 65.73{\stdfont $\pm$.87} & 54.35{\stdfont $\pm$.92} & 30.42{\stdfont $\pm$.54} & 22.17{\stdfont $\pm$.37} & 43.17 \\
    \midrule
    \multirow{4}{*}{5} & Stage1 & 48.94{\stdfont $\pm$.75} & 72.82{\stdfont $\pm$.80} & 64.74{\stdfont $\pm$.74} & 34.92{\stdfont $\pm$.53} & 21.90{\stdfont $\pm$.35} & 48.60 \\
    & Stage2 & 56.40{\stdfont $\pm$.75} & 81.61{\stdfont $\pm$.62} & 73.65{\stdfont $\pm$.72} & 37.63{\stdfont $\pm$.51} & 22.65{\stdfont $\pm$.36} & 53.89 \\
    & Stage3 & 67.07{\stdfont $\pm$.70} & 88.19{\stdfont $\pm$.57} & 80.26{\stdfont $\pm$.64} & 40.87{\stdfont $\pm$.54} & 25.25{\stdfont $\pm$.41} & \textbf{58.64} \\
    & Stage4 & \textbf{74.61{\stdfont $\pm$.65}} & 88.68{\stdfont $\pm$.53} & 75.96{\stdfont $\pm$.67} & 42.97{\stdfont $\pm$.56} & 25.80{\stdfont $\pm$.43} & 58.35 \\
    \bottomrule
\end{tabular}
}
\end{table}

\section{Results on Same-domain Target Dataset}\label{appx:same-domain_results}
\begin{table}[t!]
\small
\centering
\caption{Same-domain 5-way $k$-shot test accuracy over 600 tasks on \{miniImageNet, tieredImageNet\}.}
\label{tab:same_domain_comparison_all}
\addtolength{\tabcolsep}{-3pt}{%
\begin{tabular}{c|cc|cc}
    \toprule
     & \multicolumn{4}{c}{Dataset} \\
    \cmidrule{2-5}
     & \multicolumn{2}{c|}{miniImageNet} & \multicolumn{2}{c}{tieredImageNet} \\
     Methods & $k=1$ & $k=5$ & $k=1$ & $k=5$ \\
    \midrule
    Linear  & \textbf{51.88{\stdfont$\pm$.80}} & \textbf{74.61{\stdfont$\pm$.65}} & \textbf{61.11{\stdfont$\pm$.88}} & \textbf{80.33{\stdfont$\pm$.65}} \\
    Transfer & 44.83{\stdfont$\pm$.75} & 73.88{\stdfont$\pm$.64} & 49.49{\stdfont$\pm$.78} & 75.70{\stdfont$\pm$.70} \\
    ReFine & 49.65{\stdfont$\pm$.75} & 73.84{\stdfont$\pm$.67} & 52.26{\stdfont$\pm$.81} & 75.83{\stdfont$\pm$.69}\\
    \bottomrule
    \end{tabular} 
}
\vspace*{-8pt}
\end{table}

\section{ResNet Architecture}\label{appx:resnet_fig}
We used following backbone architectures: ResNet10 for miniImageNet, ResNet18 for ImageNet, and the extended version of ResNet18 for tieredImageNet \cite{tian2020rethinking}. 

\begin{figure}[h]
  \centering
  \includegraphics[width=.65\linewidth]{figures/sec3/resnet10.pdf}
  \caption{The structure of ResNet10 backbone network.}
  \label{fig:backbone}
\end{figure}

% \subsection*{SimCLR pre-training epochs}
% We demonstrate that the epochs of SimCLR pre-training and performance is positively correlated except for ChestX dataset.

% \begin{figure}[h]
%      \centering
%      \begin{subfigure}[h]{0.48\linewidth}
%          \centering
%          \includegraphics[width=\linewidth]{figures/sec5/perepochs/perepochs_CropDisease.pdf}
%          \caption{CropDisease}
%          \label{fig:perepochs_CropDisease}
%      \end{subfigure}
%      \hfill
%      \begin{subfigure}[h]{0.48\linewidth}
%          \centering
%          \includegraphics[width=\linewidth]{figures/sec5/perepochs/perepochs_EuroSAT.pdf}
%          \caption{EuroSAT}
%          \label{fig:perepochs_EuroSAT}
%      \end{subfigure}
     
%      \begin{subfigure}[h]{0.48\linewidth}
%          \centering
%          \includegraphics[width=\linewidth]{figures/sec5/perepochs/perepochs_ISIC.pdf}
%          \caption{ISIC}
%          \label{fig:perepochs_ISIC}
%      \end{subfigure}
%      \hfill
%      \begin{subfigure}[h]{0.48\linewidth}
%          \centering
%          \includegraphics[width=\linewidth]{figures/sec5/perepochs/perepochs_ChestX.pdf}
%          \caption{ChestX}
%          \label{fig:perepochs_ChestX}
%      \end{subfigure}
%      \caption{Fine-tuning accuracy according to SimCLR pre-training epochs.}
%      \label{fig:perepochs}
% \end{figure}

% \subsection*{5way-20shot and 5way-50shot results}
% Table XXX describes the results of 5way-20shot and 5way-50shot.

% \input{tables/comparison_only_RR_2050}

\newpage
\section{Where to Re-randomize}
\vspace{-10pt}
\begin{table}[h!]
\centering
\caption{5-way $k$-shot test accuracy over 600 tasks on miniImageNet $\rightarrow$ \{miniImageNet, BSCD-FSL\} according to the parts of re-randomization. ResNet10 is used and the mean is reported (95\% confidence interval is omitted). 0 stage indicates Transfer.}
\vspace{0.3cm}
\addtolength{\tabcolsep}{-4pt}
\resizebox{\linewidth}{!}{%
\begin{tabular}{c|c|cccc|cccccc|cccc|c}
    \toprule
    Re-randomization stage & 0 stage & \multicolumn{4}{c|}{1 stage} & \multicolumn{6}{c|}{2 stages} & \multicolumn{4}{c|}{3 stages} & 4 stages \\
    \midrule 
    Stage 1 & & \checkmark & & & & \checkmark & \checkmark & \checkmark & & & & \checkmark & \checkmark & \checkmark & & \checkmark \\
    Stage 2 & & & \checkmark & & & \checkmark & & & \checkmark & \checkmark & & \checkmark & \checkmark & & \checkmark & \checkmark \\
    Stage 3 & & & & \checkmark & & & \checkmark & & \checkmark & & \checkmark & \checkmark & & \checkmark & \checkmark & \checkmark \\
    Stage 4 & & & & & \checkmark & & & \checkmark & & \checkmark & \checkmark & & \checkmark & \checkmark & \checkmark & \checkmark \\
    \midrule
    \multicolumn{17}{l}{1-shot} \\
    \midrule
    miniImageNet  & 44.83 & 37.87 & 33.74 & 36.50 & \textbf{46.09} & 32.39 & 32.66 & 40.37 & 34.24 & 36.13 & 38.56 & 32.30 & 33.49 & 34.55 & 35.48 & 32.83 \\
    CropDisease   & 57.57 & 55.58 & 55.35 & 58.45 & \textbf{67.74} & 53.35 & 57.63 & 63.71 & 57.11 & 60.49 & 59.59 & 54.65 & 55.60 & 58.63 & 57.34 & 54.25 \\
    EuroSAT       & 51.54 & 50.00 & 49.10 & 52.83 & \textbf{63.90} & 46.89 & 49.19 & 52.35 & 49.59 & 50.76 & 53.73 & 48.20 & 47.33 & 49.80 & 49.14 & 45.70 \\
    ISIC          & \textbf{32.31} & 30.97 & 30.14 & 28.66 & 31.17 & 29.15 & 28.32 & 29.79 & 29.38 & 30.39 & 29.17 & 28.74 & 29.84 & 28.21 & 29.13 & 28.04 \\
    ChestX        & 21.82 & 21.59 & 21.31 & 21.70 & \textbf{22.46} & 21.40 & 21.92 & 21.92 & 21.89 & 21.58 & 21.75 & 21.28 & 21.51 & 21.23 & 21.15 & 20.96 \\
    \midrule
    \multicolumn{17}{l}{5-shot} \\
    \midrule
    miniImageNet  & \textbf{73.88} & 63.30 & 53.12 & 57.83 & 67.89 & 48.91 & 50.65 & 61.16 & 51.78 & 54.10 & 58.73 & 47.21 & 50.37 & 53.16 & 53.68 & 48.99 \\
    CropDisease   & 88.04 & 85.95 & 82.78 & 84.40 & \textbf{90.82} & 80.41 & 81.15 & 88.50 & 81.48 & 86.04 & 86.25 & 78.39 & 83.52 & 84.66 & 84.30 & 82.42 \\
    EuroSAT       & 79.33 & 72.61 & 71.19 & 74.79 & \textbf{81.22} & 66.86 & 69.26 & 74.15 & 70.22 & 71.27 & 74.20 & 65.97 & 64.77 & 69.20 & 69.84 & 66.23 \\
    ISIC          & \textbf{49.67} & 46.80 & 46.34 & 45.98 & 46.44 & 43.77 & 45.05 & 45.74 & 45.71 & 45.43 & 43.53 & 43.58 & 42.77 & 44.10 & 43.69 & 43.11 \\
    ChestX        & 26.10 & 24.46 & 24.51 & 25.36 & \textbf{26.50} & 23.77 & 24.48 & 25.49 & 24.18 & 24.81 & 24.23 & 23.44 & 23.89 & 24.42 & 23.68 & 23.44 \\
    \bottomrule
    \end{tabular} 
}\label{tab:where_to_reinit}
\end{table}

\begin{table}[h!]
\centering
\small
\caption{5-way $k$-shot test accuracy over 600 tasks on tieredImageNet $\rightarrow$ \{tieredImageNet, BSCD-FSL\} according to the parts of re-randomization in the last stage. ResNet18 is used and the mean is reported. Bold indicates the topmost layers.}\label{tab:where_to_reinit_in_block_tiered}
\vspace{0.3cm}
\addtolength{\tabcolsep}{-4pt}{%
\begin{tabular}{c|cccccc|cccc}
    \toprule
    {} & \multicolumn{10}{c}{Re-randomization layer} \\
    \midrule 
    Block1.Conv1          & & & & & & \checkmark & & & & \checkmark \\
    Block1.BN1            & & & & & & \checkmark & & & & \checkmark \\
    Block1.Conv2          & & & & & \checkmark & \checkmark & & & \checkmark & \checkmark \\
    Block1.BN2            & & & & & \checkmark & \checkmark & & & \checkmark & \checkmark \\
    Block1.Conv3          & & & & \checkmark & \checkmark & \checkmark & & \checkmark & \checkmark & \checkmark \\
    Block1.BN3            & & & & \checkmark & \checkmark & \checkmark & & \checkmark & \checkmark & \checkmark \\
    Block1.ShortCutConv   & & & & & & & \checkmark & \checkmark & \checkmark & \checkmark \\
    Block1.ShortCutBN     & & & & & & & \checkmark & \checkmark & \checkmark & \checkmark \\
    Block2.Conv1          & & & \checkmark & \checkmark & \checkmark & \checkmark & \checkmark & \checkmark & \checkmark & \checkmark \\
    Block2.BN1            & & & \checkmark & \checkmark & \checkmark & \checkmark & \checkmark & \checkmark & \checkmark & \checkmark \\
    Block2.Conv2          & & \checkmark & \checkmark & \checkmark & \checkmark & \checkmark & \checkmark & \checkmark & \checkmark & \checkmark \\
    Block2.BN2            & & \checkmark & \checkmark & \checkmark & \checkmark & \checkmark & \checkmark & \checkmark & \checkmark & \checkmark \\
    \textbf{Block2.Conv3} & \checkmark & \checkmark & \checkmark & \checkmark & \checkmark & \checkmark & \checkmark & \checkmark & \checkmark & \checkmark \\
    \textbf{Block2.BN3}   & \checkmark & \checkmark & \checkmark & \checkmark & \checkmark & \checkmark & \checkmark & \checkmark & \checkmark & \checkmark \\
    \midrule
    \multicolumn{11}{l}{1-shot} \\
    \midrule
    tieredImageNet& \textbf{52.26} & 50.15 & 40.30 & 36.10 & 33.89 & 31.52 & 34.42 & 35.94 & 36.64 & 33.80 \\
    CropDisease   & 67.39 & \textbf{68.31} & 60.98 & 52.84 & 48.43 & 42.61 & 51.82 & 52.78 & 51.37 & 49.28 \\
    EuroSAT       & \textbf{51.21} & 48.18 & 36.16 & 35.19 & 34.22 & 35.60 & 38.01 & 40.35 & 40.60 & 40.37 \\
    ISIC          & \textbf{28.24} & 28.06 & 27.02 & 26.64 & 26.12 & 26.94 & 26.24 & 26.35 & 26.42 & 26.70 \\
    ChestX        & \textbf{21.68} & 21.24 & 21.31 & 21.12 & 21.19 & 21.14 & 21.32 & 21.08 & 21.21 & 21.06 \\
    \midrule
    \multicolumn{11}{l}{5-shot} \\
    \midrule
	tieredImageNet& \textbf{75.83} & 75.75 & 72.61 & 64.64 & 66.44 & 62.54 & 63.40 & 61.62 & 62.59 & 62.37 \\
	CropDisease   & \textbf{90.96} & 90.84 & 90.25 & 87.25 & 86.44 & 84.06 & 83.22 & 83.00 & 84.36 & 83.17 \\
	EuroSAT       & \textbf{74.39} & 74.03 & 71.54 & 67.58 & 66.26 & 62.66 & 60.22 & 62.07 & 63.17 & 60.40 \\
	ISIC          & 38.83 & 38.76 & 37.29 & 37.85 & 38.75 & 39.85 & 37.29 & 38.35 & 39.63 & \textbf{40.91} \\
	ChestX        & 24.83 & \textbf{24.90} & 24.64 & 24.08 & 23.66 & 23.54 & 23.23 & 22.88 & 23.15 & 22.89 \\
    \bottomrule
    \end{tabular} 
}
\end{table}
